# Supplementary material for: Sparsely Overlapped Speech Training in the Time Domain: Joint Learning of Target Speech Separation and Personal VAD Benefits
Source: arXiv:2106.14371 source file (2021-09-27)

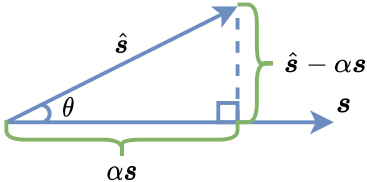

Supplement: Supplementary file 1 [file SI-SNR.pdf]
